# Supplementary material for: CanCal: Towards Real-time and Lightweight Ransomware Detection and Response in Industrial Environments
Source: arXiv:2408.16515 source file (2024-08-29)
Supplement: Supplementary file 1 [file 8.appendix_cr.tex]

\section*{Appendix}
\label{appendix}
Due to the page limit constraints of the proceedings, the full appendices of this paper, including detailed sensitivity analysis, feature distribution studies, model selection process, and additional real-world experimental results, are not included in this version. The complete version of our paper, containing all appendices and supplementary materials, is available on arXiv at \url{https://arxiv.org/abs/XXXX.XXXXX}.
